# Supplementary material for: Multi-domain improves out-of-distribution and data-limited scenarios for medical image analysis
Source: arXiv:2310.06737 source file (2024-07-04)
Supplement: Supplementary file 1 [file appendix.tex]

\clearpage
